# Supplementary material for: Counting to Four is still a Chore for VLMs
Source: arXiv:2604.10039 source file (2026-04-11)
Supplement: Supplementary file 1 [file supplement.tex]

% CVPR 2026 Supplementary Material Template

\documentclass[10pt,twocolumn,letterpaper]{article}

% For workshop submission / arXiv-style page numbers
\usepackage[pagenumbers]{cvpr}

% Import additional packages
\input{preamble}

\definecolor{cvprblue}{rgb}{0.21,0.49,0.74}
\usepackage[pagebackref,breaklinks,colorlinks,allcolors=cvprblue]{hyperref}
\usepackage{booktabs}
\usepackage{rotating}
\usepackage{adjustbox}

\title{Supplementary Material for\\
Counting to Four is still a Chore for VLMs}

\author{Duy Le Dinh Anh$^\dagger$, Patrick Amadeus Irawan$^\dagger$, Tuan Van Vo\\
MBZUAI\\
{\tt\small {\{duy.le, patrick.irawan, tuan.vo\}@mbzuai.ac.ae}}\\
{\small $^\dagger$Equal contribution.}
}

\begin{document}

\maketitle
\appendix

% Optional: restart figure/table/section numbering in supplement
\setcounter{section}{0}
\renewcommand{\thesection}{A.\arabic{section}}

% If you want section letters like A, B, C instead:
% \renewcommand{\thesection}{\Alph{section}}

\input{sec/7_Appendix}

% Add bibliography only if appendix cites new references
% {
%     \small
%     \bibliographystyle{ieeenat_fullname}
%     \bibliography{main}
% }

\end{document}
